# Supplementary material for: Polarization-dependent interference between dipole moments of a resonantly excited quantum dot
Source: arXiv:1610.06963 ancillary file (2016-10-21)
Supplement: Supplementary file 1 [file Dipole_Interference_supp_v1_0.pdf]

## Supplementary Information for

### “Polarization-dependent interference between dipole moments of a resonantly excited quantum dot”

Disheng Chen<sup>1</sup>, Gary R. Lander<sup>1</sup>, Glenn S. Solomon<sup>2</sup>, Edward B. Flagg<sup>1</sup>

<sup>1</sup>Department of Physics and Astronomy, West Virginia University, Morgantown, WV 26506, USA

<sup>2</sup>Joint Quantum Institute, National Institute of Standards and Technology,  
& University of Maryland, Gaithersburg, MD, USA.

In this Supplementary Material, we provide further information on:

- Section 1: Experimental setup & lifetime measurement
- Section 2: Theoretical model and coherence extraction
- Section 3: Stokes parameter measurement
- Section 4: Lorentzian fitting
- Section 5: Requirements for asymmetric coherence
- Section 6: Spectrum amplitude

All the figures and equations in Supplementary Information are labeled with the prefix “S” to distinguish from those that appear in the body of the Letter.

#### SECTION 1: EXPERIMENTAL SETUP & LIFETIME MEASUREMENT

The optical setup configured for polarization-dependent RPLE measurements is shown in Fig. S1(a). The sample is excited by a resonant cw laser via excitation from the side [1], and the spectral-integrated photoluminescence (PL) from the QD is collected by a CCD (charge coupled device) from the front of the sample. The orthogonal geometry and the waveguide within the sample naturally discriminate the strong excitation beam from the weak fluorescence signal by taking advantage of their different propagation directions, regardless of polarization. Thus we are able to manipulate the PL polarization via a pair of liquid crystal variable retarders (LCVRs) without being required to change the excitation polarization. However, all LCVRs show an inherent shift of the fast-axis that depends on the applied voltage and is unique to each device. This shift is usually small (less than  $5^\circ$ , see inset of Fig. S1(a)), but its complicated dependence on voltage makes it difficult to compensate for it optically. This becomes the main source of uncertainty in measuring the Mueller Matrix of the collection path.

The lifetime of the QD is measured with time-resolved fluorescence, wherein the QD is excited by 2.36 ps long

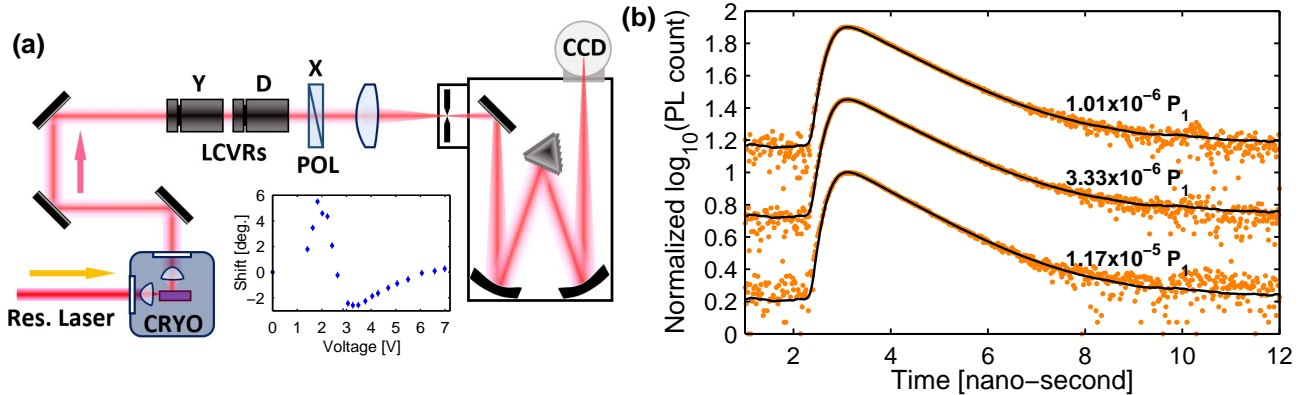

FIG. S1. (a) Experimental setup. The sample and the above-band excitation path (not shown) are the same as described in reference [1]. The spectrometer has a resolution of 0.02 nm, which is too coarse to resolve the fine structure in the QD’s emission. But it is useful to select the PL from a specific QD and remove the unwanted photons from other sources. Inset: Measured fast-axis shift for the second LCVR (D). (b) Lifetime Measurement. The orange dots are the raw data. The black curves are the fittings with an exponential decay convolved with the measured instrument response function (IRF). The power indicated is that of the weak above-band excitation required to allow resonance fluorescence; the resonant excitation power is 13  $\mu$ W. The lifetime does not vary with above-band power, and is determined to be the average of the three fitted values:  $T_1 = (570 \pm 9)$  ps.

resonant pulses centered at 927.604 nm with a time-averaged power of 13  $\mu\text{W}$ . The PL is recorded with a single photon avalanche detector ( $\tau$ -SPAD, from PicoQuant). This experiment is carried out at three different above-band-gap excitation powers:  $1.17 \times 10^{-5} P_1$ ,  $3.33 \times 10^{-6} P_1$ , and  $1.01 \times 10^{-6} P_1$ , as shown in Fig. S1(b), where  $P_1$  is the saturation power of the above-band excitation ( $P_1 = 187.5 \mu\text{W}$ ). The data are then fitted with an exponential decay convolved with the measured instrument response function (IRF). The lifetime  $T_1$  is determined to be the statistical average of these three fitting results:  $T_1 = (570 \pm 9)$  ps, since  $T_1$  shows no dependence on the above-band excitation power [1].

## SECTION 2: THEORETICAL MODEL & COHERENCE EXTRACTION

We model the system using a semi-classical Hamiltonian in the dipole and rotating wave approximations and expressed in a rotating frame with respect to the excitation laser frequency:

$$H = \sum_j \hbar \Delta_j \pi_j^\dagger \pi_j + \sum_j \frac{1}{2} \hbar \Omega_j (\pi_j^\dagger + \pi_j) \quad (\text{S1})$$

where the sum over  $j$  represents the two fine structure states;  $\Delta_j = \omega - \omega_j$  are the detunings between the laser frequency,  $\omega$ , and the fine structure states;  $\pi_j^\dagger$  and  $\pi_j$  are the raising and lowering operators for the fine structure states; and  $\Omega_j$  are the Rabi frequencies. We solve for the density matrix using a master equation in Lindblad form:

$$\dot{\rho} = \frac{1}{i\hbar} [H, \rho] + \sum_j \left[ \frac{1}{2} \Gamma_{sp} \mathcal{L}(\rho, \pi_j) + \frac{1}{2} \Gamma \mathcal{L}(\rho, \pi_j^\dagger \pi_j) \right] \quad (\text{S2})$$

In the master equation, dissipative effects are included via Lindblad super-operators for radiative decay and pure dephasing with rates  $\Gamma_{sp}$  and  $\Gamma$ , respectively:  $\mathcal{L}(\rho, O) = O\rho O^\dagger - \frac{1}{2}(\rho O^\dagger O + O^\dagger O\rho)$ .

In order to compare to the recorded RPLE data, we calculate the intensity of the emitted light as a function of the excitation frequency. The positive frequency part of the electric field operator for spontaneous emission is related to the lowering operators for the two excited states,  $\pi_1$  and  $\pi_2$  [2, 3]:

$$\mathbf{E}^{(+)}(\mathbf{r}, t) = \sum_j \frac{\omega_j^2}{8\pi^2 \epsilon_0 c^2 r} \mathbf{d}_j \pi_j \left( t - \frac{r}{c} \right) \quad (\text{S3})$$

where  $\mathbf{d}_j$  is the transition dipole moment,  $\omega_j$  is the frequency for the transition from the ground state to state  $|j\rangle$ , and  $\mathbf{r}$  is the vector from the quantum dot to the observation point. For a typical quantum dot the confinement potential is asymmetric and the exchange interaction causes the dipole moments of the fine structure states to be linearly polarized and orthogonal to each other [4–7], though of equal magnitude. The time-averaged polarization-independent and polarization-dependent total intensities of the spontaneous emission are:

$$I = \frac{1}{2} \epsilon_0 c \left\langle \mathbf{E}^{(-)}(\mathbf{r}, t) \cdot \mathbf{E}^{(+)}(\mathbf{r}, t) \right\rangle \quad (\text{S4})$$

$$I_\epsilon = \frac{1}{2} \epsilon_0 c \left\langle \left( \hat{\epsilon} \cdot \mathbf{E}^{(-)}(\mathbf{r}, t) \right) \left( \hat{\epsilon} \cdot \mathbf{E}^{(+)}(\mathbf{r}, t) \right) \right\rangle \quad (\text{S5})$$

where  $\mathbf{E}^{(-)}$  is both the negative frequency part of the electric field operator and the Hermitian adjoint of  $\mathbf{E}^{(+)}$ , and  $\hat{\epsilon}$  is the vector corresponding to the detection polarization. The angled brackets represent both ensemble averaging and time averaging. In  $I$  there will be terms proportional to  $\pi_j^\dagger \pi_j$ , but because of the orthogonality of the dipole moments the cross terms vanish. This is not the case for  $I_\epsilon$  because the dipole moments are turned into scalars via the dot product with  $\hat{\epsilon}$ . Thus, the orthogonality of the dipole moments is no longer present to eliminate cross terms such as  $\pi_1^\dagger \pi_2$ . It is important to note that the orthogonality of the dipole moments is critical to the polarization dependence of the scattered light intensity. If the dipole moments were parallel to each other, as in an atomic system with spherical symmetry, then the cross terms would be present for all detection polarizations and thus the spectrum would have the same shape for all polarizations.

The ensemble-averaged values of the operator combinations in  $I$  and  $I_\epsilon$  are equal to elements of the quantum mechanical density matrix of the system:  $\langle \pi_i^\dagger \pi_j \rangle = \rho_{ji}(t)$ . This allows us to express the detected emission intensity as a function of the density matrix elements, and we calculate those in turn using the master equation S2. The time-averaging allows us to use only the steady-state solutions to the master equation,  $\rho_{ij}^\infty$ . Depending on the detection

polarization, the functional form for  $I_\varepsilon$  will be different. Referring to Fig. 1(b), for a given choice of  $\hat{\varepsilon}$  the dot products in Eqn. S5 can be replaced by sinusoidal functions of  $\varphi$ . For X-polarized, Y-polarized, and polarization-independent detection, the functional forms are:

$$I_X = \frac{d^2\omega_0^2}{16\pi^2cr} \{ \sin^2(\varphi)\rho_{11}^\infty + \cos^2(\varphi)\rho_{22}^\infty - \sin(2\varphi)\mathcal{Re}[\rho_{12}^\infty] \} \quad (\text{S6})$$

$$I_Y = \frac{d^2\omega_0^2}{16\pi^2cr} \{ \cos^2(\varphi)\rho_{11}^\infty + \sin^2(\varphi)\rho_{22}^\infty + \sin(2\varphi)\mathcal{Re}[\rho_{12}^\infty] \} \quad (\text{S7})$$

$$I = I_X + I_Y = \frac{d^2\omega_0^2}{16\pi^2cr} \{ \rho_{11}^\infty + \rho_{22}^\infty \} \quad (\text{S8})$$

where we have approximated the two transition frequencies  $\omega_1$  and  $\omega_2$  using their average  $\omega_0 = (\omega_1 + \omega_2)/2$ , and recognized that  $\rho_{21}^\infty$  is the complex conjugate of  $\rho_{12}^\infty$ . These are the Eqns. (1), (2), and (3) that appear in the Letter.

Similarly, the RPLE intensity for other detection polarizations (diagonal (D), anti-diagonal (A), left- (L) and right-circular (R)) are:

$$I_D = \frac{d^2\omega_0^2}{32\pi^2cr} \{ \rho_{11}^\infty + \rho_{22}^\infty + (\rho_{11}^\infty - \rho_{22}^\infty) \sin(2\varphi) - 2 \cos(2\varphi) \mathcal{Re}[\rho_{12}^\infty] \} \quad (\text{S9})$$

$$I_A = \frac{d^2\omega_0^2}{32\pi^2cr} \{ \rho_{11}^\infty + \rho_{22}^\infty - (\rho_{11}^\infty - \rho_{22}^\infty) \sin(2\varphi) + 2 \cos(2\varphi) \mathcal{Re}[\rho_{12}^\infty] \} \quad (\text{S10})$$

$$I_L = \frac{d^2\omega_0^2}{32\pi^2cr} \{ \rho_{11}^\infty + \rho_{22}^\infty + 2\mathcal{Im}[\rho_{12}^\infty] \} \quad (\text{S11})$$

$$I_R = \frac{d^2\omega_0^2}{32\pi^2cr} \{ \rho_{11}^\infty + \rho_{22}^\infty - 2\mathcal{Im}[\rho_{12}^\infty] \} \quad (\text{S12})$$

where  $\hat{\varepsilon}$  for left- and right-circular polarizations is defined as  $(\hat{x} + i\hat{y})/\sqrt{2}$  and  $(\hat{x} - i\hat{y})/\sqrt{2}$ , respectively.

To extract the real part of the coherence  $\mathcal{Re}[\rho_{12}^\infty]$  from experimental data, we re-write Eqns. S6 and S7 with fitting parameters as follows:

$$I_X = A_X \{ \sin^2(\varphi)\rho_{11}^\infty + \cos^2(\varphi)\rho_{22}^\infty - \sin(2\varphi)\mathcal{Re}[\rho_{12}^\infty] \} + B_X \quad (\text{S13})$$

$$I_Y = A_Y \{ \cos^2(\varphi)\rho_{11}^\infty + \sin^2(\varphi)\rho_{22}^\infty + \sin(2\varphi)\mathcal{Re}[\rho_{12}^\infty] \} + B_Y \quad (\text{S14})$$

where  $A$  is the normalization constant and  $B$  is the background offset.  $A_X$  here is the normalization constant  $A_0$  plotted in Fig. 5 in the main text.

The data in Fig. 2(b) can be fitted with

$$I_1 = A_1\rho_{11}^\infty + B_1 \quad (\text{S15})$$

$$I_2 = A_2\rho_{22}^\infty + B_2 \quad (\text{S16})$$

allowing us to determine the populations  $\rho_{11}^\infty$  and  $\rho_{22}^\infty$ , which can then be substituted back into Eqn. S13 and S14 to solve for  $\mathcal{Re}[\rho_{12}^\infty]$ :

$$\mathcal{Re}[\rho_{12}^\infty]_X = -\frac{I_X - B_X}{A_X \sin(2\varphi)} + \frac{1}{2} \frac{I_1 - B_1}{A_1} \tan(\varphi) + \frac{1}{2} \frac{I_2 - B_2}{A_2} \cot(\varphi) \quad (\text{S17})$$

$$\mathcal{Re}[\rho_{12}^\infty]_Y = \frac{I_Y - B_Y}{A_Y \sin(2\varphi)} - \frac{1}{2} \frac{I_1 - B_1}{A_1} \cot(\varphi) - \frac{1}{2} \frac{I_2 - B_2}{A_2} \tan(\varphi) \quad (\text{S18})$$

These expressions give the extracted coherence  $\mathcal{Re}[\rho_{12}^\infty]$  plotted in Fig. 2(c) and Fig. 3.

### SECTION 3: STOKES PARAMETER MEASUREMENT

In addition to the RPLE spectra in Fig. 2(a), the other four spectra measured with the detection polarization in the D, A, L, and R directions are also recorded by choosing the appropriate LCVR voltages. These six spectra enable us to analyze the QD emission polarization via Stokes parameters. As mentioned in the Letter, the measured Mueller matrix of the collection path has been used to undo the rotation of the PL polarization state caused by the collection optics. The corrected data are shown in Fig. S2(a-c) along with simulations using parameters from the fittings in Fig. 2(a). These data directly confirm that the QD asymmetry axes are closely aligned to the diagonal and anti-diagonal directions. The red curve in Fig. S2(a) is the difference between the D and A polarization components of the fluorescence. It dominates over the curves in Fig. S2(b) and (c), which are the X-Y and L-R differences, respectively. The small but non-zero X-Y component in Fig. S2(b) is due to fact that the electric dipole moments of the QD are not perfectly aligned to diagonal or anti-diagonal directions. The non-zero L-R component in Fig. S2(c) implies elliptically polarized emission at the resonances. According to Eqns. S11 and S12, the difference ( $I_L - I_R$ ) is proportional to the imaginary part of the coherence,  $\text{Im}[\rho_{12}^\infty]$ . However, the uncertainty in the Mueller matrix causes an evident deviation of the corrected data from the simulation, and thus prevents us from accurately extracting  $\text{Im}[\rho_{12}^\infty]$  from the data.

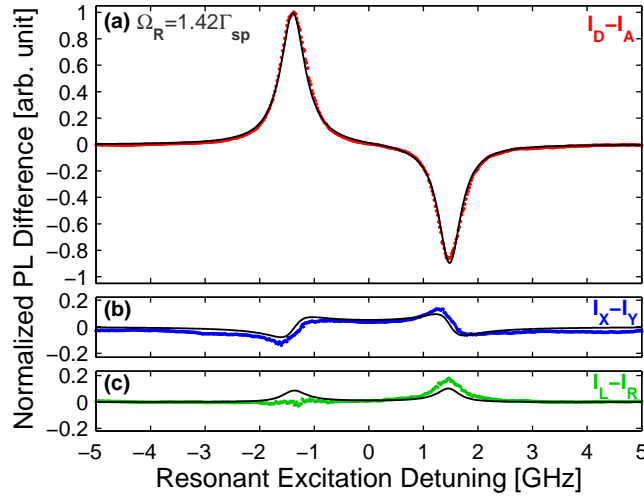

FIG. S2. Differences between RPLE spectra measured at an excitation power of  $\Omega_R = 1.42\Gamma_{sp}$ . (a) Intensity difference between D- and A-polarized spectra ( $I_D - I_A$ ). (b) Intensity difference between X- and Y-polarized spectra ( $I_X - I_Y$ ). (c) Intensity difference between left- and right- circular polarized spectra ( $I_L - I_R$ ). The black curves are simulations using parameters extracted from a fit similar to the one done in Fig. 2(a). All experimental data are normalized to the maximum intensity of the D-polarized spectrum. Before doing the subtraction between two spectra, the rotation of the polarization caused by the optics in the collection path has been corrected by inverting the Mueller matrix of the collection path upon the measured Stokes vector.

## SECTION 4: LORENTZIAN FITTING

Figure S3 shows all the RPLE spectra measured at different excitation powers and with the LCVR voltages chosen to project the excited populations  $\rho_{11}^\infty$  or  $\rho_{22}^\infty$  onto the measurement axis. The Lorentzian fits (black curves) reproduce these data successfully, implying that each excited level in the neutral QD behaves like a 2-level quantum emitter. As the resonant power increases, power broadening is apparent for both states.

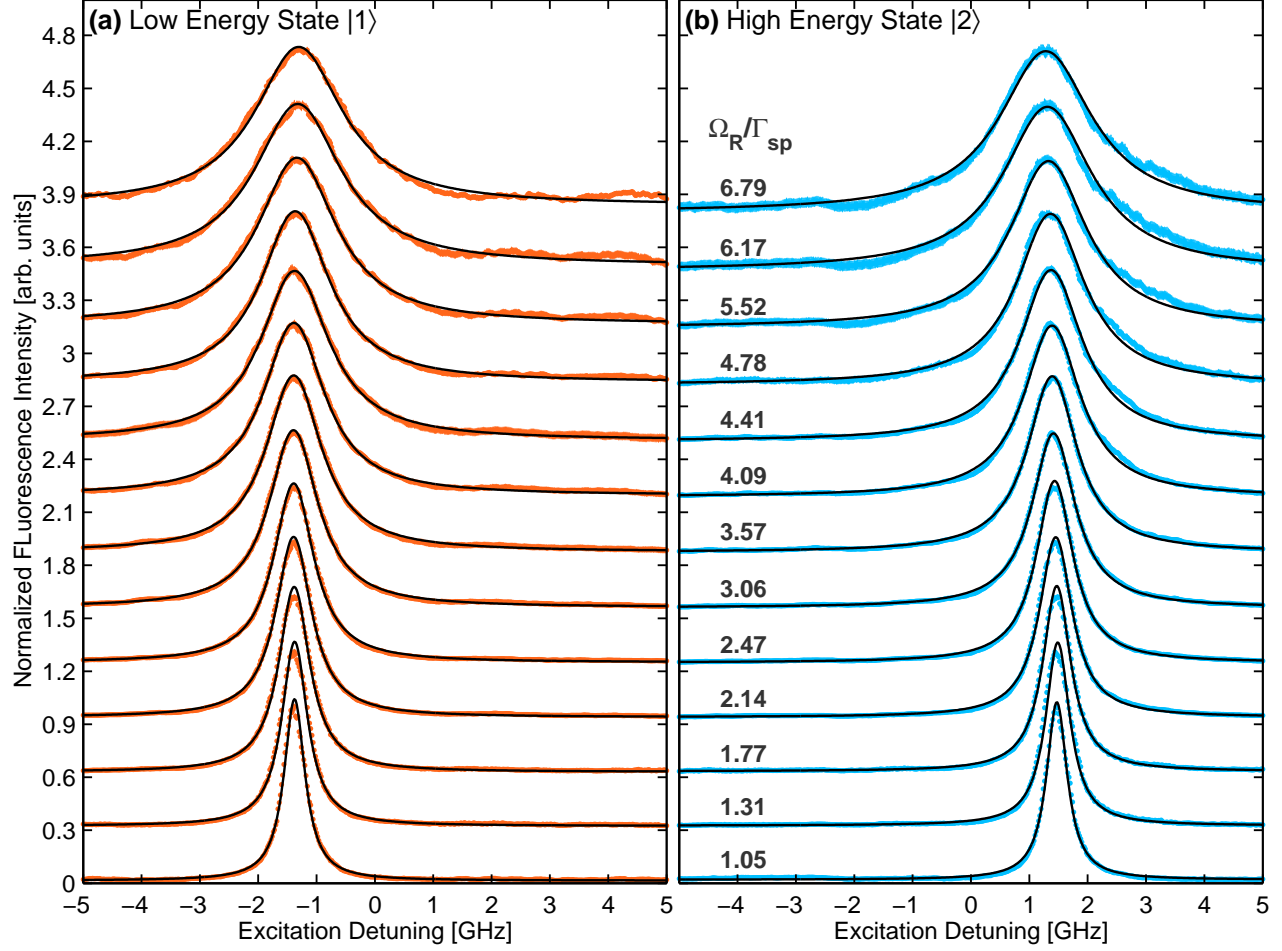

FIG. S3. Lorentzian fits to the measured populations (a)  $\rho_{11}^\infty$  and (b)  $\rho_{22}^\infty$ . The colored dots are the raw data and the black curves are fits with Lorentzian functions. All data have been normalized to their own maximum values. The curves are offset purposely for clarity. The excitation powers are labeled in the overall Rabi frequency  $\Omega_R$  in units of the population decay rate  $\Gamma_{sp}$ , following the same practice as in the Letter.

## SECTION 5: REQUIREMENTS FOR ASYMMETRIC COHERENCE

To better demonstrate the assertion in the Letter that the single condition of tilted QD axes is not sufficient to produce an asymmetric coherence, we calculate  $\mathcal{Re}[\rho_{12}^\infty]$  of a heavily tilted QD by setting  $\varphi = 10^\circ$  with respect to the excitation field  $\mathbf{E}_0$  in the Y-direction ( $\theta = 0^\circ$ ) and plot the results in Fig. S4(a). All other parameters (e.g., lifetime, fine structure splitting, etc.) are the same as in Fig. 1(a). It is clear that the coherence  $\mathcal{Re}[\rho_{12}^\infty]$  is nearly symmetric at low excitation power ( $\Omega_R = 0.579\Gamma_{sp}$ ) even when the excitation of the two energy states is uneven. As the power increases ( $\Omega_R > \Gamma_{sp}$ ),  $\mathcal{Re}[\rho_{12}^\infty]$  becomes more and more asymmetric.

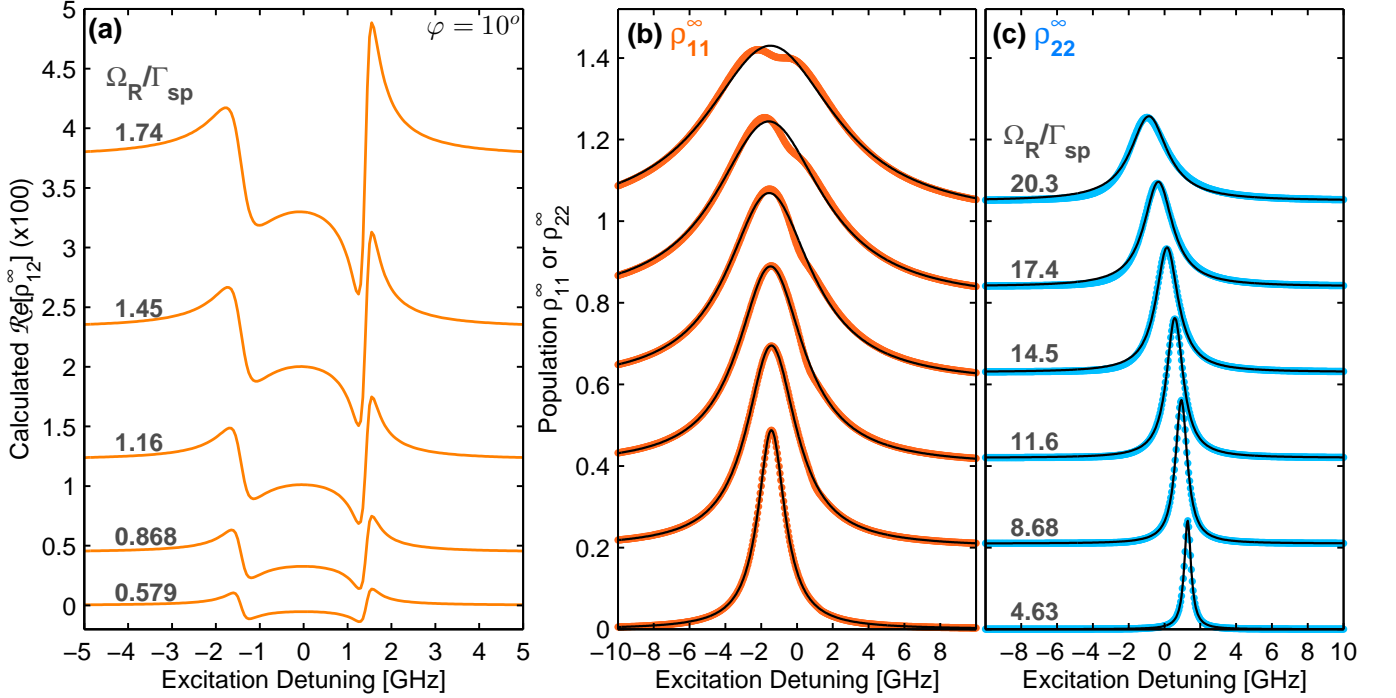

FIG. S4. (a) Calculated coherence  $\mathcal{Re}[\rho_{12}^\infty]$  by setting the QDs electric dipole moment  $\mathbf{d}_1$  to be  $10^\circ$  off from the excitation field  $\mathbf{E}_0$ . (b) Calculated population  $\rho_{11}^\infty$  in the low energy excited state  $|1\rangle$  (thick orange curves) along with the Lorentzian fit (black curves). (c) Calculated population  $\rho_{22}^\infty$  in the high energy excited state  $|2\rangle$  (thick blue curves) along with the Lorentzian fit (black curves).

When the excitation power increases such that  $\Omega_R > 10\Gamma_{sp}$ , the populations in the excited levels  $|1\rangle$  and  $|2\rangle$  also start to deviate from the symmetric Lorentzian line shape as shown in Fig. S4(b) and (c) for the calculated  $\rho_{11}^\infty$  and  $\rho_{22}^\infty$ , respectively. Since in this case the QD is tilted in favor of exciting the low energy state  $|1\rangle$ ,  $\rho_{11}^\infty$  is always larger than  $\rho_{22}^\infty$ . In addition, the excited population of the high-energy state  $\rho_{22}^\infty$  shows an evident red-shift of its peak position due to the AC Stark effect, while the peak position of the excited population of the low-energy state  $\rho_{11}^\infty$  hardly moves. This difference can be explained by noticing that the Rabi frequency  $\Omega_1$  for level  $|1\rangle$  is 5.6 times larger than the Rabi frequency  $\Omega_2$  for level  $|2\rangle$  under the same excitation power, i.e.,  $\Omega_1 = \Omega_2 \cot(\varphi) = 5.6\Omega_2$ . This leads to a stronger AC Stark effect on level  $|1\rangle$  compared to that on level  $|2\rangle$ , resulting in a clear red-shift of  $\rho_{22}^\infty$  and a nearly stationary  $\rho_{11}^\infty$ .

## SECTOIN 6: SPECTRUM AMPLITUDE

The normalization constant  $A_X$  extracted from fitting Eqns. S13 and S14 to the data in Fig. 2(a) (main letter) provides a more direct evidence on the influence of the resonant laser on the QD's local environment. The dependence of  $A_X$  on the excitation power is shown in Fig. S5. Since the V-system model completely incorporates the population variation in the excited states  $|1\rangle$  and  $|2\rangle$  for different excitation powers and detunings, one might naively expect  $A_X$  to be a constant that only depends on the exposure time and collection efficiency rather than on the resonant excitation power. However, its evident dependence upon excitation power implies that the resonant laser must also modify the fraction of time that the QD spends in the neutral state. This behavior is consistent with measurements on other QD systems [1, 8].

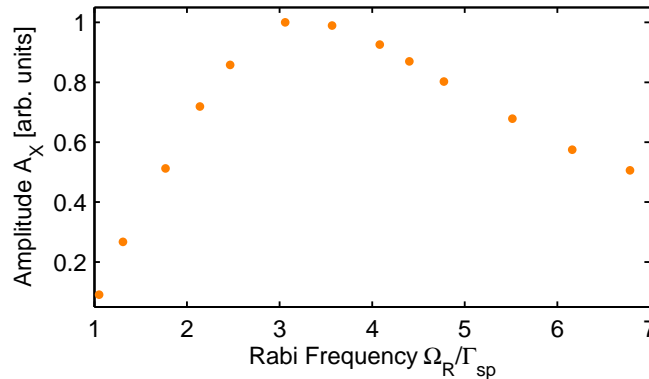

FIG. S5. Normalization factor  $A_X$  of X-polarized spectra at different excitation powers. From the fitting, the amplitude ratio of Y-polarized to X-polarized spectra is found to be  $0.799 \pm 0.003$ , which is very close the expected value (experimentally measured) of 0.8067 due to polarization-dependent absorption in the collection path.

- 
- [1] D. Chen, G. R. Lander, K. S. Krowpman, G. S. Solomon, and E. B. Flagg, *Physical Review B* **93**, 115307 (2016).
  - [2] M. O. Scully and M. S. Zubairy, *Quantum Optics* (University Press, Cambridge, U. K., 1997).
  - [3] R. Loudon, *The Quantum Theory of Light*, 3rd ed. (Oxford U. Press, 2000).
  - [4] D. Gammon, E. S. Snow, B. V. Shanabrook, D. S. Katzer, and D. Park, *Physical Review Letters* **76**, 3005 (1996).
  - [5] E. L. Ivchenko, *physica status solidi (a)* **164**, 487 (1997).
  - [6] M. Bayer, G. Ortner, O. Stern, A. Kuther, A. A. Gorbunov, A. Forchel, P. Hawrylak, S. Fafard, K. Hinzer, T. L. Reinecke, S. N. Walck, J. P. Reithmaier, F. Kloppe, and F. Schfer, *Physical Review B* **65**, 195315 (2002).
  - [7] H. Tong and M. W. Wu, *Physical Review B* **83**, 235323 (2011).
  - [8] H. S. Nguyen, G. Sallen, M. Abbarchi, R. Ferreira, C. Voisin, P. Roussignol, G. Cassabo, and C. Diederichs, *Physical Review B* **87**, 115305 (2013).
